# Supplementary material for: Portability of Fortran's `do concurrent' on GPUs
Source: arXiv:2408.07843 source file (2024-12-23)
Supplement: Supplementary file 1 [file appendix_artifact_availability.tex]

\section*{Summary of the experiments reported}

The HipFT code was built and run on NVIDIA, Intel, and AMD GPUs, as well as on CPUs.  Both server and consumer hardware was tested.  The test case is the run located in the {\tt examples/} {\tt flux\_transport\_1rot\_flowAa\_diff\_r8} folder of the HipFT github repository located at \url{https://github.com/predsci/hipft}.  The {\tt v1.11.0} release of the code was used for CPU runs and the NVIDIA and AMD GPU runs. The {\tt v1.11.0-intel-gpu} branch release (only 6 modified lines) was used for Intel GPU runs.
% \rc{and the {\tt v1.11.0-alt} branch release was used for AMD runs???}.  

\section*{Artifact Availability}

\paragraph{Software Artifact Availability:}  
All author-created software artifacts are maintained in a public repository under an OSI-approved license.

\paragraph{Hardware Artifact Availability:}  
There are no author-created hardware artifacts.

\paragraph{Data Artifact Availability: }  
All author-created data artifacts are maintained in a public repository under an OSI-approved license.

\paragraph{Proprietary Artifacts:} 
No author-created artifacts are proprietary.

\paragraph{List of URLs and/or DOIs where artifacts are available:}
\begin{Verbatim}[breaklines=true, breakanywhere=true]
https://github.com/predsci/HipFT/releases/tag/v1.11.0
https://github.com/predsci/HipFT/releases/tag/v1.11.0-intel-gpu
\end{Verbatim}
%\rc{{\tt https://github.com/predsci/HipFT/
%releases/tag/v1.11.0-alt}}
